# Supplementary material for: Distributed Symmetric Key Establishment: a Scalable Quantum-Safe Key Distribution Protocol
Source: arXiv:2407.20969 source file (2024-07-30)
Supplement: Supplementary file 1 [file app_security.tex]

\section{Additional details on composable security of DSKE}\label{app:composable_security}
\subsection{Ideal system} \label{subsec:ideal_system}

In the constructive cryptography framework, one can define an ideal system to capture desired functionalities and properties that one hopes to securely realize by the protocol of interest. In our setting with Alice, Bob, and an adversary Eve, the ideal resource should have three interfaces $A$, $B$ and $E$. It should produce a secret $S^A$ for Alice and a secret $S^B$ to Bob, which is supposed to be the same as $S^A$ in the case that the protocol completes. Given that Bob can abort in the DSKE protocol under certain conditions, we should also allow the ideal resource system to abort under the same conditions. To indicate that the protocol was aborted, the ideal system sets $S^B$ to be the symbol ${\perp}$. Security Hubs in the DSKE protocol are treated as resources in our analysis and thus are located inside the ideal resource system. As Eve can control all compromised security Hubs and all communication channels, the ideal system should give Eve the ability to control them through its $E$-interface. Each Hub can operate in one of two modes: honest or compromised. In the honest mode, the Hub simply relays the input it receives from the sender to the receiver, and does not output anything at the $E$-interface. In the compromised mode, the Hub outputs the sender's input at the $E$-interface, and uses an input from the $E$-interface to set the output of the receiver's interface.

Although not required by the framework, we can consider a particular instantiation of the ideal system to help to better understand the behaviour of this ideal system in the DSKE protocol setting. This resource system can be thought as containing a secure key resource to generate a uniformly distributed secret $S^A=S^B$, which will be distributed to Alice and Bob after checking the abort condition (if the protocol aborts, $S^B$ will be set to ${\perp}$, the flag for aborting the protocol). The ideal resource system internally contains a (modified) real resource system (see \Cref{figs:real_protocol}) that runs the skeleton DSKE protocol with the secret $S^A$ to determine the abort conditions but ignores the reconstructed secret at Bob's side. In particular, it uses the Shamir $(n,k)$-threshold scheme to generate shares by using $S^A$ as the secret. The secret-authenticating tag $o^A$ is computed using the secret $S^A$ as well as an additional key $u^A$ produced by its internal secret key resource. The ideal system gives $S^A$ as its $A$-interface's output and $S^B$ as its $B$-interface's output.

To discuss the inputs and outputs at the $E$-interface of the ideal system, we break the overall $E$-interface into the $E$-interface of each Hub $P_i$. We treat the Hub $P_i$ and its corresponding communication channels as one entity for ease of discussion and we simply say Hub $P_i$ to mean the entire entity. We use $\overline{Y}^E_i$ and $\overline{T}^E_i$ to denote inputs at the Hub $P_i$'s $E$-interface. Similarly, we use $Y^E_i$ and $T^E_i$ to denote the Hub's outputs at the $E$-interface. We use $Z^E_i\in \{00, 01, 10, 11\}$ to denote another input from the Hub $P_i$'s $E$-interface, which can be used to determine the behaviours of two authenticated channels. To fix the interpretation of values, 0 means the authenticated channel transmits the input message faithfully and 1 means it produces an error. For compromised Hubs, $\overline{Y}^E_i$ can take any allowed value for a share and $\overline{T}^E_i$ can take any allowed value for the secret-authenticating tag. A compromised Hub $P_i$ gives its share $Y_i$ and the secret-authenticating tag $o^A$ it received as the outputs to its $E$-interface, that is, $Y^E_i := Y_i$ and $T^E_i := o^A$. (Note that there might be other ancillary information to be passed to $T^E_i$. See the discussion about $T_i$ in \Cref{sec:real_system}.) We further assume $Z^E_i:=00$ for compromised Hubs since this allows Eve to fully control the compromised Hubs by $\overline{Y}^E_i$ and $\overline{T}^E_i$.  For honest Hubs, $\overline{Y}^E_i$ and $\overline{T}^E_i$ can only take the value ${\perp}$ (which is the only symbol in the allowed alphabet for those variables related to honest Hubs), indicating that Eve cannot control those honest Hubs. Honest Hubs do not leak the information about their shares and thus we set $Y^E_i := {\perp}$ for those honest Hubs. Note that since the secret-authenticating tag is not encrypted, we can simply set $T^E_i := o^A$ for honest Hubs as well. By our assumptions, we assume there is some fixed set $C \subset \{1, \dots, n\}$ with $|C| < k$, of the identifiers of all compromised Hubs.

Here we state some properties of the ideal resource system in terms of the joint probability distribution $Q_{S^A,S^B,(Y^E_i,T^E_i,\overline{Y}^E_i,\overline{T}^E_i, Z^E_i)_i}$ of the inputs and outputs at all its interfaces. This is not an exhaustive list. 
\begin{enumerate}[label=(\roman*).,leftmargin=2em]
    \item Correctness: The marginal distribution of $S^A$ and $S^B$ satisfies that for any $s^A, s^B\in F^m$ such that $s^B \neq s^A$ and $s^B \neq {\perp}$,%
    \begin{aeq}
        Q_{S^A,S^B}(s^A, s^B) = 0.
    \end{aeq}%
    \item Confidentiality: With $|C| < k$, the conditional probability distribution of $S^A$ conditioned on knowing the values of $(Y^E_j)_{j \in \mc{C}}$ as well as all $T^E_i$ satisfies%
    \begin{aeq}
        Q_{S^A|(Y^E_j)_{j \in \mc{C}}, (T^E_i)_i}=Q_{S^A}. 
    \end{aeq}%
    \item Uniform randomness: The marginal distribution of $S^A$ satisfies that for any $s \in F^m$,%
    \begin{aeq}
        Q_{S^A}(s) = \frac{1}{|F|^m}.
    \end{aeq}%
\end{enumerate}
\begin{remark}
    We note that with the instantiation of the ideal system discussed above, the correctness and uniform randomness of the ideal system are effectively due to the use of a secure key resource. The confidentiality of the ideal system is effectively due to the confidentiality provided by the Shamir $(n,k)$-threshold scheme (see \cref{thm:secret_confidentiality}) and the confidentiality provided by the secret-authenticating tag (see \cref{thm:hash_function_confidentiality}). This is because its internal modified real system runs the $(n,k)$-threshold scheme using the secret in order to abort under the same condition as the DSKE protocol.
\end{remark}

\subsection{Real system}\label{sec:real_system}

The real system is depicted in \Cref{figs:real_protocol}. In constructive cryptography, the real system uses a set of resources and converters to construct a secure equivalent of the ideal resource system.

\subsubsection{Resources}

We prove the security of the skeleton protocol assuming the availability of following resources:
\begin{enumerate}[label=(\arabic*)]
    \item Secret key resource: each user and Security Hub pair have a shared secret key resource that has only output interfaces. 
    \item Authenticated channel resource: each communication link between a user and a Security Hub is an authenticated channel.
    \item Security Hub resource: Each Security Hub can operate in one of its two modes: honest or compromised. In the honest mode, it receives $(Y_i, T_i)$ from its sender and simply sets $\overline{Y}_i := Y_i$ and $\overline{T}_i := T_i$ to give to its receiver; it ignores inputs from the $E$-interface and sets $T^E_i:=T_i$ and $Y^E_i:={\perp}$.  In the compromised mode, it receives $\overline{Y}^E_i$ and $\overline{T}^E_i$ from the $E$-interface, and sets $\overline{Y}_i :=\overline{Y}^E_i$ and $\overline{T}_i :=\overline{T}^E_i$, which are sent to its receiver; it outputs $Y_i$ and $T_i$ received from its sender to the $E$-interface, i.e., $Y^E_i:=Y_i, T^E_i := T_i$. 
\end{enumerate}
We use $\mf{R}_s$ to denote all resources used in the real system.

From a secret key resource and an authenticated channel resource we can construct a secure channel that either transmits the input message confidentially and correctly or produces the ${\perp}$ symbol to indicate an error when an adversary attempts to modify the message. We remark that in the DSKE protocol, $Y_i$ and $\overline{Y}_i$ are encrypted using the secret key resources. In \Cref{figs:real_protocol}, we use $T_i$ to denote the non-encrypted part of the message from Alice to the Hub $P_i$, and similarly $\overline{T}_i$ to denote the non-encrypted part of the message from the Hub $P_i$ to Bob. Then the encrypted version of $Y_i$ (similarly $\overline{Y}_i$) is transmitted together with $T_i$ (correspondingly $\overline{T}_i)$ in one message through an authenticated channel. 

We remark that the secret key resources are available after the one-time setup process in the DSKE protocol. However, the authenticated channel resource is not available in the general DSKE protocol. Thus, after proving the security of the skeleton protocol, we then prove the security of the general DSKE protocol by constructing an authenticated channel resource using a secret key resource and an insecure channel.

\subsubsection{Converters}

We need converters that use secret key resources and authenticated channels and $n$ Security Hub resources to (approximately) construct the ideal system. We now define converters for the DSKE protocol.

As depicted in \Cref{figs:real_protocol}, Alice has a converter $\pi^A$ that produces $S^A$, the shares $Y_i$ and a secret-authenticating tag $o^A$ for validation of the secret. Alice communicates with the Hub $P_i$ through an authenticated channel by sending the encrypted version of $Y_i$ along with $T_i$ where she sets $T_i=P_i \parallel A\parallel B \parallel o^A$, where $P_i \parallel A \parallel B$ is used for identity validation and $o^A$ is the secret-authenticating tag\footnote{Note that $T_i$ and $\overline{T}_i$ in the protocol may contain other necessary information such as the offset for the unused portion of each table and a secret identification number. We omit writing such information here for simplicity as it does not affect our discussion.}. As a result, the Hub can either receive share $Y_i$ and $T_i$ without modification or securely detect errors and get ${\perp}$ for $Y_i$ and $T_i$. Bob has a converter $\pi^B$ that receives inputs from authenticated channels from each Hub to Bob, and outputs $S^B$, which can take the value of ${\perp}$ to indicate abort of the protocol. Inside the converter $\pi^B$, it runs the secret reconstruction step and the secret validation step of the DSKE protocol.

The real system is described by a joint probability distribution $P_{S^A,S^B,(Y^E_i,T^E_i,\overline{Y}^E_i,\overline{T}^E_i, Z^E_i)_i}$.

\subsection{Distinguisher and simulator}
For $3$-interface resources, a distinguisher $\mf{D}$ is a system with $4$ interfaces, where $3$ interfaces connect to the interfaces of a resource $\mf{R}$ and the other interface outputs a bit that indicates its guess about which resource is given.

As the second condition in \cref{def:composable_security} considers the situation where Eve is active, we need to introduce a simulator $\sigma^E$ (which is Eve's converter) such that when it connects with the ideal system, the $E$-interface of $\mf{S}\sigma^E$ is the same as the $E$-interface of the real system $\pi^s\mf{R}_s$. Note that $\mc{C}$ is used to denote the set of all identifiers of compromised Security Hubs, and that $|C| \leq k-1$ under our assumptions. As Eve can fully control compromised Hubs in our threat model, the simulator $\sigma^E$ needs to have different operations for Hubs in $C$ and for Hubs in the complement set.  

We note that the $E$-interface of the ideal system accepts $(\overline{Y}^E_i, \overline{T}^E_i, Z^E_i)_i$ as inputs and produces $(Y^E_i, T^E_i)_i$ as outputs. It also gives the ability to set the operation modes of Security Hubs. In the real system shown in \Cref{figs:real_protocol}, Security Hubs whose identifiers are in the set $C$ operate in the compromised mode while the rest are in the honest mode. This means the simulator $\sigma^E$ needs to set the operation modes of those Hubs and blocks the ability to change the operation modes to match the $E$-interface of the real system. Except setting the operation modes, the $E$-interface of the simulator $\sigma^E$ is then identical to the $E$-interface of the ideal system. One possible simulator $\sigma^E$ behaves in the following way. The simulator $\sigma^E$ sets operation modes of the Security Hubs contained inside the ideal resource system. For each Hub in the set of compromised Hubs $C$, it sets the Hub $P_i$ to operate in the compromised mode and uses $Z^E_i:=00$ it receives from its $E$-interface to set the behaviours of two authenticated channels for the Hub $P_i$. For all other Hubs that are not in the set $C$, the simulator $\sigma^E$ sets the Hub $P_j$ to operate in the honest mode and uses $Z^E_j$ to set the behaviours of two authenticated channels for the Hub $P_j$. The $E$-interface of the simulator also accepts the a pair of values $(\overline{Y}^E_i,\overline{T}^E_i)$ and it outputs $(Y^E_i, T^E_i)$ received from the ideal system. The allowed alphabets for those variables are determined by the operation mode of each corresponding Hub.

\subsection{Security of the skeleton protocol}
We present some preliminaries and detailed proofs here for completeness. 

For two probability distributions $P_X$ and $Q_X$ of a random variable $X$ that can take any value in some set $\mathcal{X}$, the statistical or total variation distance between $P_X$ and $Q_X$ has the following properties:%
    \begin{aeq}\label{eq:statistical_distance_property}
        &\frac{1}{2}\sum_{x \in \mathcal{X}}|P_X(x)-Q_X(x)| \\
         = &\max_{\mathcal{X}':\mathcal{X}'\subseteq \mathcal{X}}\sum_{x \in \mathcal{X}'}(P_X(x)-Q_X(x)) \\
         = &\sum_{x: P_X(x) \geq Q_X(x)} (P_X(x)-Q_X(x)).
    \end{aeq}

    For a class of distinguishers $\mathbb{D}$, the distinguishing advantage for two resources $\mf{R}$ and $\mf{S}$ is%
\begin{aeq}\label{eq:distinguishing_advantage}
    d(\mf{R}, \mf{S}) := \max_{\mf{D} \in \mathbb{D}} (\Pr[\mf{D}\mf{R} = 1] - \Pr[\mf{D}\mf{S}=1]),
\end{aeq}%
where $\mf{D}\mf{R}$ is the binary random variable corresponding to $\mf{D}$ connected to $\mf{R}$, and $\mf{D}\mf{S}$ is defined similarly. Each binary random variable may take the value $1$ if the distinguisher $\mf{D}$ guesses the resource that it is connected to is the ideal resource system, and take the value $0$ if it guesses the real resource system\footnote{Exchanging 0 and 1 does not impact on the distinguishing advantage.}.

\begin{theorem}\label{thm:skeleton_security_repeated}
	Under the assumptions listed in \Cref{subsec:assumptions}, the protocol $\pi^s = (\pi^A, \pi^B)$ described above (depicted in \Cref{figs:real_protocol}) is $\epsilon$-secure, where $\epsilon=\min({n \choose k}\frac{m+1}{|F|},1)$, which is determined by the family of hash functions used in the protocol as described in \cref{thm:secret_validation} as well as the choices of $n$ and $k$ in the $(n, k)$-threshold scheme. 
\end{theorem}
\begin{proof}
	We need to check two conditions in \cref{def:composable_security}.

	To check the first condition, we use converters $\alpha^E$ and $\gamma^E$ to plug into the $E$-interface in the real and ideal systems. They both allow all messages $Y_i, T_i$ and $\overline{Y}_i$, $\overline{T}_i$ to be delivered correctly in authenticated channels (that is, $Z^E_i = 00$ for all $i$) and completely block $E$-interface from the distinguisher. Those two converters may still control compromised Hubs in the same predefined way with the restriction that the number of compromised Hubs is at most $k-1$. In this case, the distinguisher can observe only outputs from $A$- and $B$-interfaces.  

    We use $X$ to denote $S^A,S^B$ and use $\mathcal{X}$ to denote the set of values that $S^A,S^B$ can take. As any distinguisher can only observe $S^A$ and $S^B$, from the distinguisher's point of view, the real system is completely described by $P_{X}$ and the ideal system with the simulator $\sigma^E$ by $Q_{X}$. To guess whether it is holding the real system, a deterministic strategy for the distinguisher is that the distinguisher can pick a subset $\mathcal{X}' \subseteq \mathcal{X}$ such that for all $x \in \mathcal{X}'$, it outputs $1$ and for all other values of $x$, it outputs 0. The distinguisher may also choose a mixed (probabilistic) strategy. We note that each mixed strategy is just a probabilistic mixture of pure (deterministic) strategies. Let $\mf{D}'$ be a distinguisher that uses an arbitrary mixed strategy which is a probabilistic mixture of deterministic strategies $\mathcal{X}'_k$ with corresponding probabilities $p_k$. The distinguishing advantage of this strategy is thus bounded by%
    \begin{aeq}
        &\Pr[\mf{D}'\pi^s\mf{R}_s\alpha^E=1]-\Pr[\mf{D}'\mf{S}\gamma^E=1] \\
        =~&\sum_k p_k \sum_{x \in \mathcal{X}'_k} (P_X(x) - Q_X(x))\\
        \leq~& \sum_k p_k \Big[\max_{\mathcal{X}':\mathcal{X}'\subseteq \mathcal{X}}\sum_{x \in \mathcal{X}'} (P_X(x) - Q_X(x))\Big]\\
        =~&\max_{\mathcal{X}':\mathcal{X}'\subseteq \mathcal{X}}\sum_{x \in \mathcal{X}'} (P_X(x) - Q_X(x)),
    \end{aeq}%
    where the first equality is due to the chosen strategy of the distinguisher $\mf{D}'$, which can be written as a probabilistic mixture of deterministic strategies, the inequality is due to the fact that we perform an optimization over all subsets $\mathcal{X}'$ of $\mathcal{X}$ and $\mathcal{X}'_k$ is just a possible subset of $\mathcal{X}$, and the last equality is the result of summing over $k$. Thus, it is enough to consider all deterministic strategies. 

    In this case, the distinguishing advantage is%
 	\begin{aeq}\label{eq:ske_metric_calculation}
		&d(\pi^s\mf{R}_s\alpha^E,\mf{S}\gamma^E)  \\
        =~& \max_{\mf{D} \in \mathbb{D}}(\Pr[\mf{D}\pi^s\mf{R}_s\alpha^E=1]-\Pr[\mf{D}\mf{S}\gamma^E=1]) \\
        =~& \max_{\mathcal{X}':\mathcal{X}'\subseteq \mathcal{X}}\sum_{x \in \mathcal{X}'} (P_X(x) - Q_X(x)) \\
        =~& \frac{1}{2}\sum_{x \in \mathcal{X}}  |P_{X}(x) - Q_{X}(x)|, \\
    \end{aeq}%
    where the first equality is due to the definition of the pseudo-metric in \cref{eq:distinguishing_advantage}, the second equality is due to the general deterministic strategy of the distinguisher as described above and that the optimal value of the distinguishing advantage can always be realized by a deterministic strategy, and the third equality is due to \cref{eq:statistical_distance_property}. We see that the distinguishing advantage is related to the statistical distance between $P_X$ and $Q_X$. 

    Our task is then to evaluate the statistical distance. We note that the allowed alphabets for $\overline{Y}^E_i$ and $\overline{T}^E_i$ depend on whether $i \in \mc{C}$. For ease of writing, we do not explicitly write out alphabets for those variables.  
    For any value of $s^A$ and any value of $s^B$ such that $s^B \neq s^A$ and $s^B \neq \perp$, the joint probability distribution of the ideal system $Q_{X}(s^A, s^B) = 0$, while the joint probability distribution of the real system $P_{X}(s^A, s^B) \neq 0$ due to the correctness of secret validation being approximate, which depends on the property of hash functions used for the secret-authenticating tag as in \cref{thm:secret_validation}. When restricting to all possible values of $(s^A, s^B)$ such that $P_X(s^A, s^B)> Q_X(s^A, s^B)$, the real and ideal systems differ only in the case where the real system may obtain $s^B \neq s^A$ and $s^B \neq \perp$. To see this, we show the contrapositive: if $s^A=s^B$ or $s^B =\perp$, then $P_{X}(s^A, s^B) \leq Q_{X}(s^A, s^B)$. For each $s^A$, we observe (i) $P_{S^A}(s^A) = Q_{S^A}(s^A) = \frac{1}{|F|^m}$, (ii) $P_{X}(s^A, \perp) = Q_{X}(s^A, \perp)$ and (iii) for each $s^B \neq s^A$, $Q_{X}(s^A, s^B) = 0$ while $P_{X}(s^A, s^B) \geq 0$. As we can write
    \begin{aeq}
P_{S^A}(s^A) &= \sum_{s^B} P_X(s^A, s^B)\\ &=  \sum_{s^B \neq \perp} P_X(s^A, s^B)  +  P_X(s^A, \perp),   
    \end{aeq}% 
    and
        \begin{aeq}
Q_{S^A}(s^A) &= \sum_{s^B} Q_X(s^A, s^B) \\&=  Q_X(s^A, s^A)  +  Q_X(s^A, \perp),
    \end{aeq}%
    these two equations imply $P_X(s^A, s^A) \leq Q_X(s^A, s^A)$ for each $s^A$ following those facts (i)-(iii).

    Thus, the distinguishing advantage is% 

    \begin{flalign}
		&d(\pi^s\mf{R}_s\alpha^E,\mf{S}\gamma^E) \nonumber &\\
		=~& \sum_{x: P_X(x) \geq Q_X(x)} (P_X(x) - Q_X(x)) \label{eq:cond1_ske_calc_distance_property} &\\
		=~& \sum_{s^A} \sum_{s^B: s^B \neq s^A, s^B \neq \perp} P_{X}(s^A, s^B) \label{eq:cond1_ske_calc_P_Q_properties} &\\
		=~& \sum_{s^A, (\overline{y}_i, \overline{t}_i)_i}  \sum_{\substack{s^B: s^B \neq s^A, \\ s^B \neq \perp}}P_{S^A, S^B, (\overline{Y}^E_i, \overline{T}^E_i)_i}(s^A, s^B, (\overline{y}_i, \overline{t}_i)_i) \label{eq:cond1_ske_cal_sum_over_yt} &\\
		=~& \sum_{s_A, (\overline{y}_i, \overline{t}_i)_i} P_{S^A, (\overline{Y}^E_i, \overline{T}^E_i)_i}(s^A, (\overline{y}_i, \overline{t}_i)_i) \nonumber &\\
		& \times   \sum_{ \substack{s^B: s^B \neq s^A,\\ s^B \neq \perp}} P_{S^B|S^A, (\overline{Y}^E_i, \overline{T}^E_i)_i}(s^B | s^A, (\overline{y}_i, \overline{t}_i)_i) \label{eq:cond1_ske_cal_convert_to_conditional_prob}, &
	\end{flalign}%
    where we use \cref{eq:statistical_distance_property} to obtain \cref{eq:cond1_ske_calc_distance_property} from \cref{eq:ske_metric_calculation}, we obtain \cref{eq:cond1_ske_calc_P_Q_properties} since the condition $P(x)\geq Q(x)$ is equivalent to the situation where Bob does not abort the protocol and Bob obtains $S^B$ that is different from $S^A$ as discussed above (also note $Q_X(x) = 0$ for such $x$), we write the marginal probability $P_{S^A, S^B}$ in terms of summing $P_{S^A, S^B, (\overline{Y}^E_i, \overline{T}^E_i)_i}$ over all possible values of $(\overline{Y}^E_i, \overline{T}^E_i)_i$ to get \cref{eq:cond1_ske_cal_sum_over_yt}, and we finally rewrite the joint probability over $S^A, S^B, (\overline{Y}^E_i, \overline{T}^E_i)_i$ by the conditional probability $P_{S^B | S^A, (\overline{Y}^E_i, \overline{T}^E_i)_i}$ and the marginal probability $P_{S^A, (\overline{Y}^E_i, \overline{T}^E_i)_i}$ to obtain \cref{eq:cond1_ske_cal_convert_to_conditional_prob}.

    Under the assumption that at most $k-1$ Hubs are compromised, we can safely assume whenever $S^B \neq \perp$, the secret-authenticating tag $o^A$ is transmitted faithfully from at least $k$ Hubs to Bob. The reason is that Bob would set $S^B$ to $\perp$ and abort the protocol if fewer than $k$ Hubs send the same secret-authenticating tag; on the other hand, to agree on a value $t \neq \perp$ other than $o^A$ for the secret-authenticating tag, at least $k$ Hubs need to send the same modified value $t$, which is not possible given that at most $k-1$ Hubs are compromised. Thus, for each value of $s^A, (\overline{y}_i, \overline{t}_i)_i$,%
    \begin{aeq}\label{eq:con_prob_epsilon_estimation}
        & \sum_{ \substack{s^B: s^B \neq s^A, \\ 
        s^B \neq \perp}} P_{S^B|S^A, (\overline{Y}^E_i, \overline{T}^E_i)_i}(s^B | s^A, (\overline{y}_i, \overline{t}_i)_i) \\
    	\leq & \min({n \choose k}\Pr[h_{u'}(s^B) = o^A|s^A, (\overline{y}_i, \overline{t}_i)_i, s^B \neq s^A], 1) \\
    	\leq &  \min({n \choose k}\frac{m+1}{|F|},1)=:\epsilon,
    \end{aeq}%
    where $u' \parallel s^B$ is the secret reconstructed from a subset of $\{\overline{y}_i\}$ with $k$ elements, the factor ${n \choose k}$ is due to there being up to {${n \choose k}$} possible values of $u'\parallel s^B$ that the secret validation step can check, and we use \cref{thm:secret_validation} (where we remove the freedom to choose $t'$ and set $t'=0$) for the last inequality.%
    \footnote{The multiplier ${n \choose k}$ may significantly reduce the security for large $n$.  For example, $n=99$, $k=50$ results is a security loss of $\log {99\choose 50}=95.35\text{ bits}$.  For $n\le11$, the security loss is under 9 bits, but with Bob still having to search up to ${11 \choose 6}=462$ combinations.  A protocol variant, which we do not elaborate, allows Bob to filter out bad shares before combining them, at the cost of several tags per share.}

    Combining \cref{eq:cond1_ske_cal_convert_to_conditional_prob,eq:con_prob_epsilon_estimation}, we have%
    \begin{aeq}
    	&d(\pi^s\mf{R}_s\alpha^E,\mf{S}\gamma^E) \\
    	\leq & \sum_{s_A, (\overline{y}_i, \overline{t}_i)_i} P_{S^A, (\overline{Y}^E_i, \overline{T}^E_i)_i}(s^A, (\overline{y}_i, \overline{t}_i)_i) \epsilon
    	= \epsilon.
    \end{aeq}%
    This verifies the first condition in \cref{def:composable_security}.

    To check the second condition, we consider the simulator $\sigma^E$ as depicted in \Cref{figs:ideal+simulator}. In this case, Eve's interface allows the distinguisher to control all compromised Hubs. A distinguisher can pick any allowed value of $(\overline{Y}^E_i, \overline{T}^E_i, Z^E_i)_i$ as an input to the system and observe $S^A, S^B, (Y^E_i, T^E_i)_i$ from outputs of the unknown system. The restriction on the number of compromised Hubs is reflected by different alphabets of $\overline{Y}^E_i$, $\overline{T}^E_i$ and $Z^E_i$ for $i \in \mc{C}$ and for $i \in \{1, \dots, n\}\setminus\mc{C}$. The real system is completely characterized by $P_{S^A,S^B,(Y^E_i,T^E_i,\overline{Y}^E_i,\overline{T}^E_i, Z^E_i)_i}$ and the ideal system with the simulator $\sigma^E$ is completely characterized by $Q_{S^A,S^B,(Y^E_i,T^E_i,\overline{Y}^E_i,\overline{T}^E_i, Z^E_i)_i}$. We now use $X$ to denote $S^A,S^B,(Y^E_i,T^E_i,\overline{Y}^E_i,\overline{T}^E_i, Z^E_i)_i$ and let $\mathcal{X}$ denote the set of values that $S^A,S^B,(Y^E_i,T^E_i,\overline{Y}^E_i,\overline{T}^E_i, Z^E_i)_i$ can take.

    We note that the ideal system and the real system abort under the same condition since the ideal system internally runs the DSKE protocol to determine abort conditions. Therefore, for any allowed value $s^A, (y_i, t_i, \overline{y}_i, \overline{t}_i, z_i)_i$ for $(Y^E_i,T^E_i,\overline{Y}^E_i,\overline{T}^E_i, Z^E_i)_i$,%
    \begin{aeq}
    	P_{X}(s^A, \perp, (y_i, t_i, \overline{y}_i, \overline{t}_i, z_i)_i) = Q_{X}(s^A, \perp, (y_i, t_i, \overline{y}_i, \overline{t}_i, z_i)_i).
    \end{aeq}%

    By a similar argument as for the first condition, it is enough to consider all deterministic strategies when we calculate the pseudo-metric for these two systems. To guess that it is holding the real system, the distinguisher can pick a subset $\mathcal{X}' \subseteq \mathcal{X}$ such that for all $x \in \mathcal{X}'$, it outputs $1$ and for all other values of $x$, it outputs 0. (Note that we reuse the same notation as in the proof of the first condition since the proof of the second condition resembles the first one. However, $X, \mathcal{X}$ here denote a different combination of symbols and a different set, respectively.) The distinguishing advantage is
    \begin{flalign}
		&  d(\pi^s\mf{R}_s,\mf{S}\sigma^E) \nonumber &\\
		= & \sum_{x: P_X(x) \geq Q_X(x)} (P_X(x) - Q_X(x)) \label{eq:ske_calc_distance_property} &\\
		= & \sum_{\substack{s^A, \\ (y_i, t_i, \overline{y}_i, \overline{t}_i, z_i)_i}} \sum_{ \substack{s^B: s^B \neq s^A,\\ s^B \neq \perp}} P_{X}(s^A, s^B, (y_i, t_i, \overline{y}_i, \overline{t}_i, z_i)_i) \label{eq:ske_calc_P_Q_properties} &\\
		= & \sum_{s^A, (\overline{y}_i, \overline{t}_i, z_i)_i}  \sum_{\substack{s^B: s^B \neq s^A, \\ s^B \neq \perp}}P_{S^A, S^B, (\overline{Y}^E_i, \overline{T}^E_i, Z^E_i)_i}(s^A, s^B, (\overline{y}_i, \overline{t}_i, z_i)_i) \label{eq:ske_cal_sum_over_yt}&\\
		=& \sum_{s_A, (\overline{y}_i, \overline{t}_i,z_i)_i} P_{S^A, (\overline{Y}^E_i, \overline{T}^E_i, Z^E_i)_i}(s^A, (\overline{y}_i, \overline{t}_i)_i, z_i) \nonumber &\\
		& \times   \sum_{ \substack{s^B: s^B \neq s^A,\\ s^B \neq \perp}} P_{S^B|S^A, (\overline{Y}^E_i, \overline{T}^E_i, Z^E_i)_i}(s^B | s^A, (\overline{y}_i, \overline{t}_i, z_i)_i) \label{eq:ske_cal_convert_to_conditional_prob}, &
	\end{flalign}%
    where we obtain \cref{eq:ske_calc_P_Q_properties} since the condition $P(x)\geq Q(x)$ is equivalent to the situation where Bob does not abort the protocol and Bob obtains $S^B$ that is different from $S^A$ as discussed above (also note $Q_X(x) = 0$ for those $x$'s), to get \cref{eq:ske_cal_sum_over_yt}, we directly sum over all possible values of $(Y^E_i, T^E_i)_i$ since those are outputs from $E$-interface that are not used for the secret validation step, and we finally rewrite the joint probability over $S^A, S^B, (\overline{Y}^E_i, \overline{T}^E_i, Z^E_i)_i$ by the conditional probability $P_{S^B | S^A, (\overline{Y}^E_i, \overline{T}^E_i, Z^E_i)_i}$ and the marginal probability $P_{S^A, (\overline{Y}^E_i, \overline{T}^E_i, Z^E_i)_i}$ to obtain \cref{eq:ske_cal_convert_to_conditional_prob}. 

    We note that \cref{eq:con_prob_epsilon_estimation} also holds when we condition on the additional input choices $(Z^E_i)_i$ that determine the behaviours of authenticated channels since \cref{eq:con_prob_epsilon_estimation} was proved under the choice $Z^E_i =00$ for all $i$ and we considered all possible combinations of $u' \parallel s^B$ that can go through to the secret validation step when we estimated that upper bound. By setting any of $(Z^E_i)_i$ to any value other than $00$, Eve effectively reduces the number of combinations of $u' \parallel s^B$ to feed into the secret validation step while the probability for each combination of $u' \parallel s^B$ to pass the secret validation step is unchanged. In other words, for each allowed value $s^A, (\overline{y}_i, \overline{t}_i, z_i)_i$ of $S^A, (\overline{Y}^E_i, \overline{T}^E_i, Z^E_i)_i$,%
    \begin{aeq}\label{eq:cond2_cond_prob_estimation}
        & \sum_{ \substack{s^B: s^B \neq s^A, \\ 
        s^B \neq \perp}}P_{S^B|S^A, (\overline{Y}^E_i, \overline{T}^E_i, Z^E_i)_i}(s^B | s^A, (\overline{y}_i, \overline{t}_i, z_i)_i) \leq \epsilon.
    \end{aeq}%

    By using \cref{eq:cond2_cond_prob_estimation}, the distinguishing advantage is then%
    \begin{aeq}\label{eq:skeleton_secrecy_metric_calculation}
    	&d(\pi^s\mf{R}_s,\mf{S}\sigma^E) \\
    	=& \sum_{s_A, (\overline{y}_i, \overline{t}_i, z_i)_i} P_{S^A, (\overline{Y}^E_i, \overline{T}^E_i, Z^E_i)_i}(s^A, (\overline{y}_i, \overline{t}_i, z_i)_i) \\
    	& \times   \sum_{ \substack{s^B: s^B \neq s^A,\\ s^B \neq \perp}} P_{S^B|S^A, (\overline{Y}^E_i, \overline{T}^E_i, Z^E_i)_i}(s^B | s^A, (\overline{y}_i, \overline{t}_i, z_i)_i) \\
    	\leq & \sum_{s_A, (\overline{y}_i, \overline{t}_i, z_i)_i} P_{S^A, (\overline{Y}^E_i, \overline{T}^E_i, Z^E_i)_i}(s^A, (\overline{y}_i, \overline{t}_i, z_i)_i) \epsilon
        = \epsilon.
    \end{aeq}%
	
	Therefore, the second condition is also verified. Thus, the protocol is $\epsilon$-secure.
\end{proof}
\begin{remark}
    The secret validation step relies on the correctness of the secret-authenticating tag as stated in \cref{thm:secret_validation}. In the limit that $|F|\to\infty$, we have that $\epsilon\to0$, and the secret validation step is perfectly correct. In this case, the skeleton DSKE protocol perfectly constructs the ideal system out of the real resource system. 
\end{remark}

\subsection{Robustness of the skeleton protocol}\label{sec:skeleton_robustness}

Robustness of a protocol is the condition that the protocol does not abort when Eve is passive (restricted to modifying the messages of compromised Hubs only), as defined in \Cref{subsec:threat_model}.  We say a protocol is $\epsilon$-robust if its aborting probability is at most $\epsilon$ in the case of this restriction. 
When restricted in this way, the aborting probability for the skeleton DSKE protocol is at most $\epsilon=\min({n \choose k}\frac{m+1}{|F|},1)$ when the number of honest Security Hubs is at least $k$ and the number of compromised Security Hubs is at most $k-1$.\footnote{The second condition becomes significant when $2k\le n$, due to multiple competing reconstructed secrets.}
\begin{theorem}[Robustness of a skeleton DSKE protocol]\label{thm:robustness_skeleton}
	Under the assumptions listed in \Cref{subsec:assumptions}, when the upper bound on the number of compromised Security Hubs is no greater than $\min(n-k, k-1)$, the skeleton DSKE protocol is $\epsilon$-robust with $\epsilon = \min({n \choose k} \frac{m+1}{|F|}, 1)$.
\end{theorem}
\begin{proof}
	When Eve is passive, all authenticated channels in the skeleton DSKE protocol faithfully transmit messages. We note that a message using a fake identity gets rejected by the receiver without consuming any secret key resources by the assumption that a communication link provides the originating identity to the receiver. In other words, Eve cannot impersonate an honest Security Hub by using compromised Hubs to mount an attack to exhaust data in a table shared by a Security Hub and a user.
 
    If the number of honest Security Hubs is at least $k$ (which means the number of compromised Hubs cannot be more than $n-k$) and the number of compromised Hubs is at most $k-1$, the only condition that causes Bob to abort is when there are multiple different candidate tuples $(u^A, s^A, o^A)$ that pass the secret validation step. That is, in addition to the correct secret reconstructed using shares from $k$ honest Security Hubs, there must exist at least one different secret candidate that also passes the secret validation step. For each possible guess of the $(u^A, s^A)$ other than the correct secret, it can pass the secret validation step with a probability at most $\min(\frac{m+1}{|F|},1)$ due to \cref{thm:secret_validation}. Since there are at most ${n \choose k}$ valid candidates to go through the secret validation step, the aborting probability in this case is at most $\min({n \choose k}\frac{m+1}{|F|},1)=: \epsilon$. Thus, the skeleton DSKE protocol is $\epsilon$-robust when the upper bound on the number of compromised Security Hubs is no greater than $\min(n-k, k-1)$.
\end{proof}

\subsection{Security of the general DSKE protocol}\label{sec:proof}
We summarize a few useful properties of the distinguishing advantage. The distinguishing advantage defined in \Cref{eq:distinguishing_advantage} is a pseudo-metric on the set of resources. It is non-increasing under (serial or parallel) composition of any two systems, that is, for any resource systems $\mf{R}, \mf{S}, \mf{T}$, and any converter $\alpha$ (with $\alpha^i$ denoting $\alpha$ converting interface $i$),%
\begin{aeq}\label{eq:metric_serial_composition}
    d(\alpha^i\mf{R}, \alpha^i\mf{S})& \leq d(\mf{R}, \mf{S}),\\
\end{aeq}%
and%
\begin{aeq}\label{eq:metric_parallel_composition}
    d(\mf{R} \parallel \mf{T}, \mf{S} \parallel \mf{T}) &\leq d(\mf{R}, \mf{S}),\\
    d(\mf{T} \parallel \mf{R}, \mf{T} \parallel \mf{S}) &\leq d(\mf{R}, \mf{S}).\\
\end{aeq}%

We state the composability theorem from \cite{Maurer2011}, which will be useful to prove the security of the general DSKE protocol.
\begin{theorem}[{\cite[Theorem 1]{Maurer2011}}]\label{thm:composability}
	The security definition in \cref{def:composable_security} is generally composable if the pseudo-metric $d$ is compatible with the cryptographic algebra\footnote{We refer to \cite{Maurer2011} for the definitions of cryptographic algebra and compatibility of the pseudo-metric with cryptographic algebra. The pseudo-metric used in this paper is compatible with the underlying cryptographic algebra since we consider information-theoretic security so that if a distinguisher in the set of all distinguishers $\mathbb{D}$ is composed with another arbitrary system, it is still in $\mathbb{D}$. To avoid further distraction, we omit this definition here.}. The following statements hold:
	\begin{enumerate}[label=(\roman*)]
		\item If a protocol $\pi$ securely constructs a system $\mf{S}$ out of a system $\mf{R}$ within $\epsilon$ and another protocol $\pi'$ securely constructs a system $\mf{T}$ out of a system $\mf{S}$ within $\epsilon'$, then the serial composition $\pi\pi'$(running the protocol $\pi'$ after the protocol $\pi$) securely constructs the system $\mf{T}$ out of the system $\mf{R}$ within $\epsilon+\epsilon'$, i.e.,%
        \begin{aeq}
			& (\mf{R} \xrightarrow{(\pi, \epsilon)} \mf{S}) \;\land\; (\mf{S} \xrightarrow{(\pi', \epsilon')} \mf{T}) \\
            \implies & \mf{R} \xrightarrow{(\pi\pi', \epsilon+\epsilon')} \mf{T};
		\end{aeq}%
		\item If a protocol $\pi$ securely constructs a system $\mf{S}$ out of a system $\mf{R}$ within $\epsilon$ and another protocol $\pi'$ securely constructs a system $\mf{S}'$ out of a system $\mf{R}'$ within $\epsilon'$, then the parallel composition $\pi \parallel \pi'$ securely constructs the system $\mf{S} \parallel \mf{S}'$ out of the system $\mf{R} \parallel \mf{R}'$ within $\epsilon+\epsilon'$, i.e.,%
        \begin{aeq}
			& (\mf{R} \xrightarrow{(\pi, \epsilon)} \mf{S}) \;\land\; (\mf{R}' \xrightarrow{(\pi', \epsilon')} \mf{S}') \\
            \implies & \mf{R}\parallel\mf{R}' \xrightarrow{(\pi\parallel\pi', \epsilon+\epsilon')} \mf{S} \parallel \mf{S}';
        \end{aeq}%
        \item When a trivial converter, which applies the identity transformation to the resource that it connects to, is applied to a system $\mf{R}$, it perfectly constructs the system $\mf{R}$ out of itself, i.e.,%
        \begin{aeq}
            \mf{R} \xrightarrow{(\mathbf{1}, 0)} \mf{R},
        \end{aeq}%
        where $\mathbf{1}$ denotes the trivial converter.
	\end{enumerate}
\end{theorem}

To assist our discussion here, as shown in \Cref{figs:real_protocol}, we denote the secure key resource between Alice and the Hub $P_i$ as $\mbf{K}_{AP_i}$, the authenticated channel between Alice and the Hub $P_i$ as $\mbf{A}^{+}_{AP_i}$, the secure key resource between the Hub $P_i$ as $\mbf{K}_{P_iB}$, and the authenticated channel between the Hub $P_i$ and Bob as $\mathbf{A}^{+}_{P_iB}$. In the previous section, we have shown that $\pi^s$ securely constructs the ideal resource $\mf{S}$ out of $\mf{R}_s$ within $\epsilon$, where the real resource $\mf{R}_s$ in the skeleton DSKE protocol is defined as%
\begin{aeq}
	\mf{R}_s := & \mbf{K}_{AP_1} \parallel \mbf{A}^{+}_{AP_1} \parallel P_1 \parallel \mbf{K}_{P_1B} \parallel \mbf{A}^{+}_{P_1B}\parallel \dots \\
    & \parallel \mbf{K}_{AP_n} \parallel \mbf{A}^{+}_{AP_n} \parallel P_n \parallel\mbf{K}_{P_nB} \parallel \mbf{A}^{+}_{P_nB}.  
\end{aeq}%

The difference between a skeleton protocol and a general protocol using the same $(n, k)$-threshold scheme is the availability of authenticated channel resources. In a general DSKE protocol, we need to use a secure key resource and an insecure channel to construct an authenticated channel. An authentication protocol $\pi^{\auth}_{AP_i}$ (also $\pi^{\auth}_{P_iB}$) using a Carter--Wegman universal hash function family to produce message tags can securely construct an authenticated channel out of a secret key resource and an insecure channel within $\epsilon':=\min(\frac{s}{|F|},1)$ as shown in \Cref{thm:hash_function_correctness}. To distinguish this secret key resource from the secret key resource used in the skeleton protocol, we denote the new secret key resource by $\mbf{K}^{\auth}$ and the insecure channel by $\mbf{C}$ (with suitable subscripts). We then define the resource $\mf{R}_g$ used in the general DSKE protocol as%
\begin{aeq}
	\mf{R}_g :=& \; \mbf{K}_{AP_1} \parallel \mbf{K}^{\auth}_{AP_1} \parallel \mbf{C}_{AP_1} \parallel P_1 \\ & \parallel
    \mbf{K}_{P_1B} \parallel \mbf{K}^{\auth}_{P_1B} \parallel \mbf{C}_{P_1B}  \parallel \dots \\ & \parallel \mbf{K}_{AP_n} \parallel \mbf{K}^{\auth}_{AP_n} \parallel \mbf{C}_{AP_n} \parallel P_n \\ &\parallel \mbf{K}_{P_nB} \parallel \mbf{K}^{\auth}_{P_nB} \parallel \mbf{C}_{P_nB} . 
\end{aeq}%

Recall that $m$ is the length of the secret to be agreed and $s$ is the length of the message for which a tag is produced. We now show that the general DSKE protocol is $(\epsilon + 2n \epsilon')$-secure, where $\epsilon = \min({n \choose k}\frac{m+1}{|F|}, 1)$ and $\epsilon' = \min(\frac{s}{|F|},1)$.

\begin{theorem}
	The protocol $\pi^g = (\pi^s, \pi^{\auth}_{AP_1}, \dots, \pi^{\auth}_{AP_n}, \pi^{\auth}_{P_1B}, \dots \pi^{\auth}_{P_nB})$ securely constructs the ideal resource $\mf{S}$ out of the resource $\mf{R}_g$ within $\epsilon + 2n \epsilon'$, where each of $\pi^{\auth}_{AP_i}$ and $\pi^{\auth}_{P_iB}$ securely construct authenticated channels $\mbf{A}^+_{AP_i}$, $\mbf{A}^+_{P_iB}$ within $\epsilon'$, respectively, where $\epsilon = \min({n \choose k}\frac{m+1}{|F|}, 1)$ and $\epsilon' = \min(\frac{s}{|F|},1)$. 
\end{theorem}
\begin{proof}
	We start with showing the first condition in \cref{def:composable_security} where no adversary is present. We trivially have%
	\begin{aeq}
		\pi^{\auth}(\mbf{K}^{\auth}\parallel\mbf{C}) \alpha^E = \mbf{A}^{+} \beta^E
	\end{aeq}%
    for each choice of subscript ($AP_i$ or $P_iB$), where $\alpha^E$ and $\beta^E$ emulate an honest behaviour at Eve's interfaces, since both systems are equivalent to a channel that faithfully transmits a message between two parties (either $A$ and $P_i$ or $P_i$ and $B$). With a slight abuse of notation, we use $\alpha^{E^{2n}}$ and $\beta^{E^{2n}}$ to denote systems that emulate an honest behaviour at Eve's interfaces in $\pi^g\mf{R}_g$ and $\pi^s\mf{R}_s$, which include $2n$ authentication channels in the systems $\mf{R}_g$ and $\mf{R}_s$, respectively. We use $\gamma^{E^{2n}}$ to denote the system that emulates an honest behaviour at Eve's interfaces in $\mf{S}$. Thus,%
	\begin{aeq}
		& d(\pi^g \mf{R}_g \alpha^{E^{2n}}, \mf{S}\gamma^{E^{2n}}) \\
		\leq & d(\pi^g \mf{R}_g\alpha^{E^{2n}}, \pi^s \mf{R}_s \beta^{E^{2n}}) + d( \pi^s \mf{R}_s \beta^{E^{2n}}, \mf{S}\gamma^{E^{2n}})\\
		= &~ d( \pi^s \mf{R}_s \beta^{E^{2n}}, \mf{S}\gamma^{E^{2n}})	\leq \epsilon, 
	\end{aeq}%
    where the last inequality is shown in \cref{thm:skeleton_security}.
	
    We now analyze the case of an active adversary as required in the second condition in \cref{def:composable_security}. 
    As each of $\pi^{\auth}_{AP_i}$ and $\pi^{\auth}_{P_iB}$ securely construct authenticated channels $\mbf{A}^+_{AP_i}$, $\mbf{A}^+_{P_iB}$ within $\epsilon'$, respectively, there exist converters $\sigma^E_{AP_i}$ and $\sigma^E_{P_iB}$ such that%
    \begin{aeq}
        d(\pi^{\auth}_{AP_i}(\mbf{K}^{\auth}_{AP_i}\parallel\mbf{C}_{AP_i}), \mbf{A}_{AP_i}^+\sigma^E_{AP_i} ) \leq \epsilon',\\
        d(\pi^{\auth}_{P_iB}(\mbf{K}^{\auth}_{P_iB}\parallel\mbf{C}_{P_iB}), \mbf{A}_{P_iB}^+\sigma^E_{P_iB} ) \leq \epsilon'.
    \end{aeq}%
    We use $\sigma^{E}_{AP_iB}$ to denote  $\sigma^E_{AP_i} \parallel\sigma^E_{P_iB}$ and use $\sigma^{E^n}_{APB}$ to denote $n$-copies of $\sigma^{E}_{AP_iB}$ composed in parallel. For the ease of writing, we use a shorthand notation $\mbf{A}^{+}_{AP_iB}$ to denote $\mbf{A}^{+}_{AP_i} \parallel \mbf{A}^{+}_{P_iB}$ and use $\{\mbf{A}^{+}_{AP_iB}\}$ to denote $\mbf{A}^{+}_{AP_1B} \parallel \dots \parallel \mbf{A}^{+}_{AP_nB}$. Similarly, we use $\pi^{\auth}_{AP_iB}(\mbf{KC})$ to denote $\pi^{\auth}_{AP_i}(\mbf{K}^{\auth}_{AP_i} \parallel \mbf{C}_{AP_i}) \parallel \pi^{\auth}_{P_iB}(\mbf{K}^{\auth}_{P_iB} \parallel \mbf{C}_{P_iB})$. 
  
    From the properties of the pseudo-metric, we have%
    \begin{aeq}\label{eq:auth_2n_channel}
        d(\pi^g\mf{R}_g, \pi^s\mf{R}_s\sigma^{E^n}_{APB}) &\leq d(\{\pi^{\text{auth}}_{AP_iB}(\mbf{KC)}\}, \{\mbf{A}^{+}_{AP_iB}\sigma^E_{AP_iB}\})  \\
        & \leq \sum_{i=1}^n d(\pi^{\text{auth}}_{AP_iB}(\mbf{KC)}, \mbf{A}^{+}_{AP_iB}\sigma^E_{AP_iB}) \\
        & \leq 2n \epsilon',
    \end{aeq}%
    where we use \cref{eq:metric_serial_composition,eq:metric_parallel_composition} for the first inequality to remove common systems in $\pi^g\mf{R}_g$ and $\pi^s\mf{R}_s\sigma^{E^n}_{APB}$, \cref{thm:composability} for the second inequality and the security of the authentication protocol for the third inequality and the fact that there are $2n$ uses of the authentication protocol. 

    From \cref{thm:skeleton_security}, we also have a converter $\sigma^E$ such that%
    \begin{aeq}\label{eq:skeleton_secrecy}
        d(\pi^s\mf{R}_s, \mf{S}\sigma^E ) \leq \epsilon.
    \end{aeq}%
    Thus, we show that for the converter $\sigma'^E = \sigma^E \sigma^{E^n}_{APB}$, we have%
    \begin{aeq}
        &~ d(\pi^g\mf{R}_g, \mf{S}\sigma'^E) \\
        \leq &~ d(\pi^g\mf{R}_g, \pi^s\mf{R}_s\sigma^{E^n}_{APB}) + d(\pi^s\mf{R}_s\sigma^{E^n}_{APB}, \mf{S}\sigma^E\sigma^{E^n}_{APB}) \\
        \leq &~ d(\pi^g\mf{R}_g, \pi^s\mf{R}_s\sigma^{E^n}_{APB}) + d(\pi^s\mf{R}_s, \mf{S}\sigma^E)\\
        \leq &~ 2n\epsilon' + \epsilon,
    \end{aeq}%
    where we use the triangle inequality in the first inequality, \cref{eq:metric_serial_composition,eq:metric_parallel_composition} to drop the common system $\sigma^{E^n}_{APB}$ in the second inequality, and \cref{eq:auth_2n_channel,eq:skeleton_secrecy} in the third inequality.

    Combining those two conditions, we show that $\pi^g$ securely constructs the ideal resource $\mf{S}$ out of the resource $\mf{R}_g$ within $\max(\epsilon, \epsilon + 2n \epsilon')=\epsilon + 2n \epsilon'$.
\end{proof}

We then show the $\epsilon$-robustness of the general DSKE protocol.
\begin{theorem}[Robustness of a general DSKE protocol]\label{thm:robustness_general}
    When the upper bound on the number of compromised Security Hubs is no greater than $\min(n-k, k-1)$, a general DSKE protocol is $\epsilon$-robust with $\epsilon = \min({n \choose k} \frac{m+1}{|F|}, 1)$.
\end{theorem}
\begin{proof}
    When Eve is passive, a general DSKE protocol behaves in the same way as its corresponding skeleton protocol. The reason is as follows. A general DSKE and its corresponding skeleton protocol differ in the availability of authenticated channels. In the general DSKE protocol, an authentication protocol constructs an authenticated channel out of a secret key resource and an insecure channel, while in the skeleton protocol, authenticated channels are assumed to be available. When Eve is passive, she does not tamper each communication channel. Each authenticated channel in the skeleton protocol and each channel constructed by the authentication protocol in the general protocol both faithfully transmit messages. Thus, the result of \cref{thm:robustness_skeleton} directly applies.
\end{proof}

%\begin{figure*}[t]
%	\includegraphics[width=0.9\linewidth]{./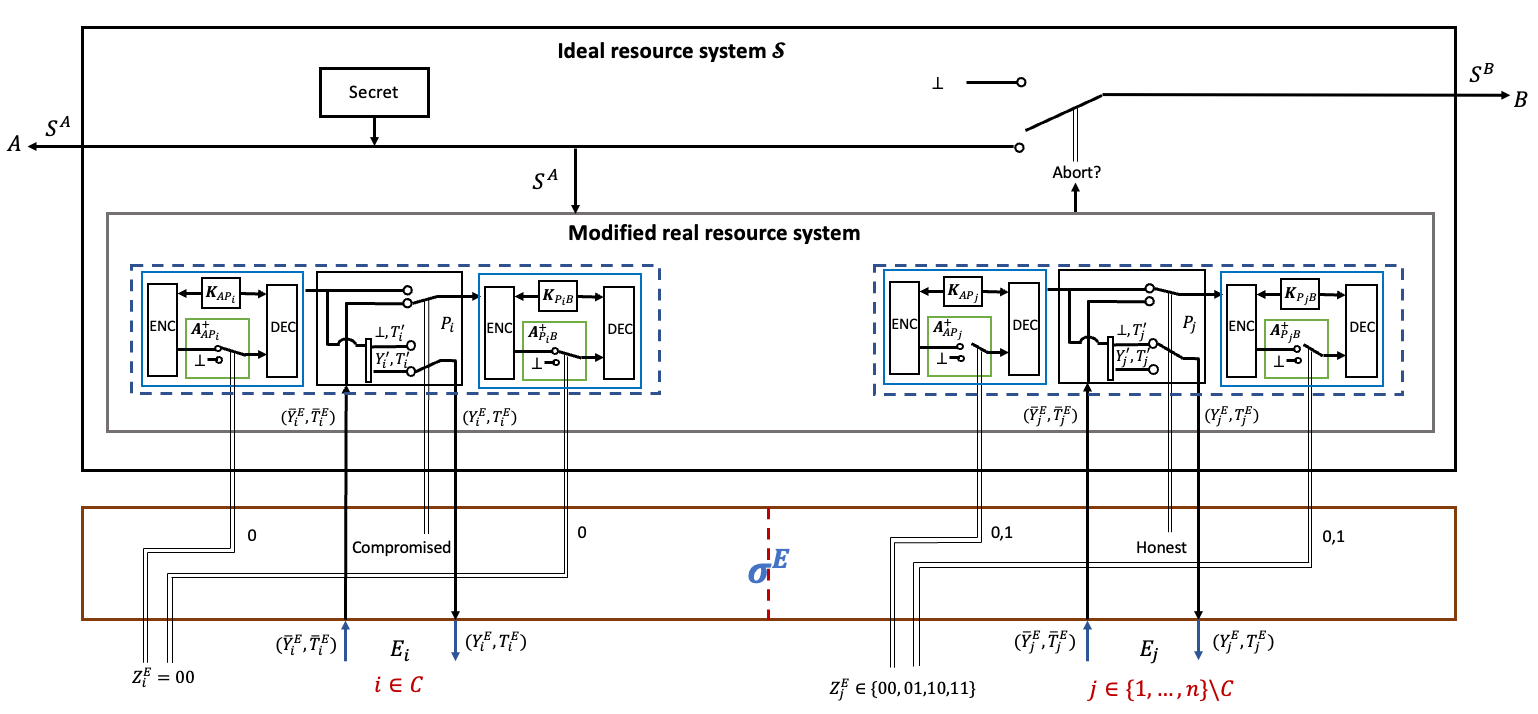}
%	\caption{An ideal key agreement resource using $n$ Security Hubs with the simulator $\sigma^E$. Hubs are reordered for drawing purposes only. The simulator $\sigma^E$ sets operation modes of the Security Hubs contained inside the ideal resource system. For each Hub in the set of compromised Hubs $C$, it sets the Hub $P_i$ to operate in the compromised mode and uses $Z^E_i:=00$ it receives from its $E$-interface to set the behaviours of two authenticated channels for the Hub $P_i$. For all other Hubs that are not in the set $C$, the simulator $\sigma^E$ sets the Hub $P_j$ to operate in the honest mode and uses $Z^E_j$ to set the behaviours of two authenticated channels for the Hub $P_j$. The $E$-interface of the simulator also accepts the a pair of values $(\overline{Y}^E_i,\overline{T}^E_i)$ and it outputs $(Y^E_i, T^E_i)$ received from the ideal system. The allowed alphabets for those variables are determined by the operation mode of each corresponding Hub.}
%	\label{figs:ideal+simulator}
%\end{figure*}
