# Supplementary material for: Distributed Symmetric Key Establishment: a Scalable Quantum-Safe Key Distribution Protocol
Source: arXiv:2407.20969 source file (2024-07-30)
Supplement: Supplementary file 2 [file notation.tex]

\section{Full list of Notation} 
\label{app:notation}

\begin{table}[!ht]
    \begin{center}
%    \resizebox{0.88\linewidth}{!}{
    \begin{tabular}{|c|l|}
    	\hline
    	\textbf{Symbol} & \textbf{Description} \\
    	\hline
    	$A$ & reference to Alice, or shorthand for $A_i$ \\
    	\hline
    	$A_i$ & Hub $P_i$'s identifier for Alice \\
    	\hline
    	$f$ & polynomial over field $F$ \\
    	\hline
    	$g$	& bijective mapping $\{0,\dots,|F|-1\} \to F$ \\
    	\hline
    	$\mathbf{H}$	& family of 2-universal hash functions \\
    	\hline
        $\mathbf{H}'$	& family of 2-universal hash functions \\
    	\hline
    	$h'_{u^A}$	& function in $\mathbf{H}'$ selected by $u^A$ \\
    	\hline
    	$h_{v^A_i}$ & function in $\mathbf{H}$ selected by $v^A_i$ \\
    	\hline
    	$H^A_i$	 & first table, for Hub $P_i$ and Alice \\
    	\hline
    	$\overline{H}^A_i$ &	second table, for Hub $P_i$ and Alice \\
    	\hline
    	$H^B_i$ &	first table, for Hub $P_i$ and Bob \\
    	\hline
    	$\overline{H}^B_i$ &	second table, for Hub $P_i$ and Bob \\
    	\hline
    	$i$	& $i\in\{1,\dots,n\}$ is a share (Hub) index. \\
    	\hline
    	$j^A_i$	& index into $H^A_i$ \\
    	\hline
    	$\overline{j}^B_i$ & index into $\overline{H}^B_i$ \\
    	\hline
    	$k$	& threshold for the sharing scheme \\
    	\hline
    	$K^A$ 	&	identifier that tracks the current $S^A$ \\
    	\hline
    	$m$	 & number of field elements in $S^A$ \\
    	\hline
    	$M^A_i$	 & message from Alice to Hub $P_i$, no tag \\
    	\hline
    	$\overline{M}^B_i$ &	message from Hub $P_i$ to Bob, no tag \\
    	\hline
    	$n$	& number of Hubs (and hence shares) \\
    	\hline
    	$o^A$ &	secret-authenticating tag for $S^A$ \\
    	\hline
    	$P_i$	& identifier referring to the $i$th Hub \\
    	\hline
    	$R^A_i$	 & $3+m$ field elements of $H^A_i$ \\
    	\hline
    	$\overline{R}^B_i$ & $3+m$ field elements of $\overline{H}^B_i$ \\
    	\hline
    	$S^A$	& Alice's secret of $m$ field elements \\
    	\hline
    	$t^A_i$	& message tag for $M^A_i$ using $v^A_i$ \\
    	\hline
    	$\overline{t}^B_i$	& message tag for $\overline{M}^B_i$ using $\overline{v}^B_i$ \\
    	\hline
    	$u^A$	& $3$ field elements of $Y^A_i$ for $o^A$ \\
    	\hline
    	$v^A_i$	& $2$ field elements of $H^A_i$ for $t^A_i$	 \\
    	\hline
    	$\overline{v}^B_i$	& $2$ field elements of $\overline{H}^B_i$ for $\overline{t}^B_i$ \\
    	\hline
    	$x_i$	& $x$-coordinate for Hub $P_i$ \\
    	\hline
    	$Y^A_i$	& $3+m$ field elements: $u^A\parallel S^A$ \\
    	\hline
    	$Z^A_i$	& encrypted $Y^A_i$ in the message $M^A_i$ \\
    	\hline
    	$\overline{Z}^B_i$	& encrypted $Y^A_i$ in the message $\overline{M}^B_i$ \\
    	\hline
    \end{tabular}
%    }
    \end{center}
    \caption{\label{table:symbols}Symbols used in the protocol description in \Cref{subsec:dske_detailed}. \textit{Note}: Symbol capitalization may differ from the main text.}
\end{table}

We define some common notations used throughout this paper to assist our discussions. In particular, $A$ refers to Alice, $B$ refers to Bob, $E$ refers to Eve, and $P_i$ refers to the unique identifier assigned to the Security Hub indexed by $i\in\{1,\dots,n\}$. We highlight that $F$ denotes the same finite field throughout, $|F|$ is the number of elements in $F$, and by \textit{element} we mean an element of $F$. By \textit{length}, we mean \textit{number of field elements}. 

As we often need to write a collection of symbols, (\dots, $Y_i$, \dots), where the index $i$ iterates through each element of a list $S$, we define a shorthand notation $(Y_i)_{i \in S}$ or simply $(Y_i)_{i}$ when the list $S$ is clear from the context (e.g., we write $(Y_1,Y_2,Y_3)$ as $(Y_i)_{i \in [1,2,3]}$ or just $(Y_i)_{i}$). We use capital letters (e.g., $Y$) to denote random variables and lowercase letters (e.g., $y$) to denote a particular value of the random variable. We use \textit{uniform} to mean \textit{uniformly distributed}. We use $\delta_{x,y}$ to denote the Kronecker delta function. Between two sequences, $\parallel$ denotes the concatenation operation. Between two resources, $\parallel$ denotes the parallel composition operation.

Throughout, given a finite sample space $\Omega$ and a probability distribution $p$ over it, we construct the corresponding probability space $(\Omega, \mathcal{F}, \mbf{P})$ by setting the event space $\mathcal{F}$ as the collection of all subsets of $\Omega$, and $\mbf{P}(A)=\sum_{\omega\in A} p(\omega)$.

\Cref{table:symbols} in lists symbols related to the protocol description. Other notations are introduced where they first appear.

% \subsection{Notation}\label{subsec:notation}
