# Supplementary material for: Distributed Symmetric Key Establishment: a Scalable Quantum-Safe Key Distribution Protocol
Source: arXiv:2407.20969 source file (2024-07-30)
Supplement: Supplementary file 3 [file security_hashing_messages.tex]

\section{Security of hashing for messages} \label{app:hash_message}

Consider a family of polynomial functions, where $c$, $d$ and $v_{j}$ are elements of a finite field $F$ \cite[Section 4.2]{Bernstein2007}:%
\begin{aeq}
    \mbf{H}=\{h_{c,d}\colon{}F^{s}\to{}F\colon{}(v_{1},\dots,v_{s})\mapsto{}d+\sum_{j=1}^{s}c^{j}v_{j}\}
\end{aeq}%
\Cref{thm:message_correctness} gives the best guessing probability that Eve's message $\mbf{v}^{*}$ is both modified from $\mbf{v}$ and validates against any tag $t^{*}$ with the selection of the hash function $h_{c,d}$ unknown, excluding the case of an empty message ($s=0$).

\begin{theorem}\label{thm:message_correctness} ~ \\
    Denote $\mbf{v} = (v_{1},\dots,v_{s})$ and $\mbf{v}^{*} = (v^{*}_{1},\dots,v^{*}_{s})$. \\
    Let $\Omega=F^2$ be a sample space with uniform probability. \\
    Let $h_{C,D}(\mbf{v})=D+\sum_{j=1}^{s}C^{j} v_{j}$ define a family of functions with random variables $(C,D)\in\Omega$ as selection parameters. 
    Let $s\ne0$. Let $t\in F$ be given.
    Then, $\max_{t^{*},\mbf{v}^{*}\ne\mbf{v}} \Pr(t^{*}=h_{C,D}(\mbf{v}^{*})~|~t=h_{C,D}(\mbf{v})) = \min(\frac{s}{|F|},1)$.
\end{theorem}
\begin{proof}
    We are given that $t=h_{C,D}(\mbf{v})$. This may be written%
    \begin{aeq}\label{eq:thm_message_correctness_a}
        t=D+\sum_{j=1}^{s}C^{j} v_{j}.
    \end{aeq}%
    This constraint serves to eliminate all pairs $(C,D)$ that do not solve \cref{eq:thm_message_correctness_a}. For every value of $C$ in $F$, this equation determines a unique value for $D$, resulting in exactly $|F|$ pairs that meet the constraint.  Conversely, for every value of $D$, there may be many values of $C$, and by inference, there may be many values of $D$ for which there is no corresponding solution for $C$. Since the \textit{a priori} probability on $\Omega$ (prior to imposing the constraint) is uniform, and each value for $C$ occurs in a pair exactly once, the \textit{a posteriori} marginal distribution on $C$ (i.e. given the constraint) is uniform, but the marginal distribution on $D$ is potentially nonuniform.

    To obtain the probability that $t^{*}=h_{C,D}(\mbf{v}^{*})$ holds, we subtract from it the given \cref{eq:thm_message_correctness_a} to obtain an equivalent equation%
    \begin{aeq}\label{eq:thm_message_correctness_b}
        t^{*}-t=\sum_{j=1}^{s}C^{j} (v^{*}_{j}-v_{j}).
    \end{aeq}%

    For any values of $t$, $t^{*}$, $\mbf{v}$ and $\mbf{v}^{*}\ne\mbf{v}$, the polynomial equation \cref{eq:thm_message_correctness_b} has up to $\min(s,|F|)$ solutions for $C$, with the bound attainable for some $\mbf{v}^{*}$.  Since $C$ is uniform, each solution has probability $\frac{1}{|F|}$.  Thus with $s\ne0$,%
    \begin{aeq}
        \max_{t^{*},\mbf{v}^{*}\ne\mbf{v}} \Pr(t^{*}-t=\sum_{j=1}^{s}C^{j}(v^{*}_{j}-v_{j}))=\min\big(\frac{s}{|F|},1\big)
    \end{aeq}%
    It follows from the equivalence with \cref{eq:thm_message_correctness_a} that%
    \begin{aeq}
        \max_{t^{*},\mbf{v}^{*}\ne\mbf{v}} \Pr(t^{*}=h_{C,D}(\mbf{v}^{*})~|~t=h_{C,D}(\mbf{v}))=\min\big(\frac{s}{|F|},1\big).
    \end{aeq}%
\end{proof}
