# Supplementary material for: Distributed Symmetric Key Establishment: a Scalable Quantum-Safe Key Distribution Protocol
Source: arXiv:2407.20969 source file (2024-07-30)
Supplement: Supplementary file 4 [file security_secret_sharing.tex]

\section{Security of validated secret sharing} \label{app:hash_secret}

\subsection{Share manipulation in secret sharing}

We use a prime to denote an associated additive difference variable. For example, $a'$ denotes a difference (error), used to produce $a+a'$ from $a$.

\begin{lemma} \label{lem:sum_independence}
    Let $\Omega=F^2$ be a sample space with $(D,X)\in\Omega$. Let $D$ and $X$ be independent random variables with $D$ uniform. Let $z\in F$ be arbitrary. \\
    Then $\Pr(D+X=z)=\frac{1}{|F|}$.
\end{lemma}
%\begin{proof}
%    For any $z\in F$,%
%    \begin{aeq}
%        &\Pr(D+X=z) & \\
%        &    = \sum_{x\in F}\Pr(D+X=z|X=x)\Pr(X=x) & \\
%        &    = \sum_{x\in F}\frac{1}{|F|}\Pr(X=x)  &  \\
%        &    = \frac{1}{|F|}.    & 
%    \end{aeq}%
%\end{proof}

\begin{lemma}\label{lem:indepsum}
    Let $\Omega=F^2$ be a sample space. Let random variables $(D,X)\in\Omega$ be mutually independent and $D$ uniform.
    Then $X+D$ and $X$ are mutually independent.
\end{lemma}
%\begin{proof}
 %   For each $(x,d) \in \Omega$,%
  %  \begin{aeq}
   %     &\Pr((X+D,X) = (x+d,x)) \\
    %    = ~& \Pr((D,X)=(d,x)) & [\text{since }X=x] \\ 
     %   = ~& \Pr(D=d)\Pr(X=x) & [\text{independence of } \\
      %  & & D\text{ and }X] \\
       % = ~& \frac{1}{|F|}\Pr(X=x) & [\text{uniformity of }D] \\
        %= ~& \Pr(X+D=x+d)\Pr(X=x) & [\text{by \cref{lem:sum_independence}}].
    %\end{aeq}%
    %By \cref{eq:prob_independent}, it follows that $X+D$ and $X$ are mutually independent.
%\end{proof}

Consider an $(n,k)$-threshold Shamir secret sharing scheme that uses a polynomial over the field $F$.

\begin{theorem}\label{thm:shamir_linearity}
% Note: this commented-out part is an early attempt at a more rigorous statement of the theorem.
%    Denote $Y_U=(Y_{1},\dots,Y_{k})$; $U=[1,\dots,k]$. \\
%    Let each $x_j\in F$ be unique for $j\in U$. \\
%    Let $Y_j\in F$ be mutually independent and uniform. \\
%    Let $\forall j\in U\colon Y_j=\sum_{i=1}^{k}C_i{x_j}^i$ for some $C_i$ (sharing). \\
    In a Shamir secret sharing scheme with threshold $k$, for any given set of $k$ shares, the secret is a linear combination of the shares.
\end{theorem}
\begin{proof}
    A Shamir scheme is based on a polynomial $f$ of degree (at most) $k-1$ over $F$, where $1\le{k}\le{n}<|F|$. In such a scheme, $n+1$ distinct $x$-coordinate values are chosen, with one ($x_{0}$) associated with the secret and the rest ($x_{1},\dots,x_{n}$) each associated with a share.  The secret sharing scheme is defined by the polynomial in $x$ as%
    \begin{aeq}
        f(x)=\sum_{j=0}^{k-1}c_{j}x^{j},
    \end{aeq}%
    with secret coefficients $c_j$.  The $c_j$ and $x_i$ determine the secret $y_0$ and shares $y_{1},\dots,y_{n}$ through $y_i=f(x_i)$.  Any $k$ of the $n+1$ pairs $(x_i, y_i)$ uniquely determine the $c_j$.  The $y_i$ for $k$ of the shares are required to be independent and uniform in $F$.
    For any $J\subseteq\{1,\dots,n\}$ with $|J|=k$, the polynomial $f$ can be expressed as a linear combination of a Lagrange basis of $k$ polynomials $L_j$ of degree $k-1$, such that $L_i(x_j)=\delta_{i,j}$ for $i,j\in{}J$:%
    \begin{aeq}
        f(x)=\sum_{i\in J}y_{i}L_{i}(x).
    \end{aeq}%
    Given known $x_i$ and a set $J$ as defined above, the basis polynomial $L_i$ corresponding to $x_i$ can be determined.  Since each polynomial $L_i$ is of degree $k-1$ and has $k-1$ distinct zeros, $L_i(x_j)\ne0$ whenever $j\not\in{}J$, and in particular, $L_i(x_0)\ne0$.  From this, the secret is a known linear combination of any given $k$ of the $n$ shares:%
    \begin{aeq}
        y_{0}=f(x_{0})=\sum_{i\in J}y_{i}L_i(x_{0}).
    \end{aeq}%
    The confidentiality of $y_0$ provided by the Shamir scheme relies on at least $n-k+1$ of the $n$ shares remaining secret.  Further, if a value $y_i+y'_i$ is substituted for each share $y_i$, the reconstructed secret is%
    \begin{aeq}
        \sum_{i\in J}(y_{i}+y'_{i})L_i(x_{0})=y_{0}+\sum_{i\in J}y'_{i}L_{i}(x_{0}).
    \end{aeq}%
    From this it may be seen that, because the $L_i(x_0)$ are known and nonzero, a single error value $y'_i=y'_0/L_i(x_0)$ added to $y_i$ replaces the reconstructed secret with $y_0+y'_0$.  With multiple errors $y'_i$, $y'_0=\sum_{i\in J}y'_iL_i(x_0)$ can be chosen by an adversary who is able to choose $y'_i$ for a nonempty subset of $J$.
\end{proof}

\subsection{Confidentiality of Shamir sharing scheme}
The fundamental confidentiality of the Shamir secret sharing scheme is expressed in \cref{thm:shamir_confidentiality} \cite{shamir1979share}.
\begin{theorem}\label{thm:shamir_confidentiality}
    In a Shamir secret sharing scheme with threshold $k$, the shared secret is independent of any subset of the shares of size $k-1$ or less.
\end{theorem}
\begin{proof}
    Let $J\subseteq\{1,\dots,n\}$, with $|J|=k$, and $i\in J$.
    From \cref{thm:shamir_linearity}, the secret $Y_0$ is a linear sum of $k$ shares:%
    \begin{aeq}
        Y_0=\sum_{j\in J}d_{j}Y_{j},
    \end{aeq}%
    where each coefficient $d_{j}=L_{j}(x_{0})$ is nonzero for all $j\in J$. In a Shamir sharing scheme each subset of $k-1$ shares is mutually independent and uniform. The secret $Y_{0}$ can therefore be partitioned into a sum for any $i\in{}J$:%
    \begin{aeq}
        Y_{0}=d_{i}Y_{i}+\sum_{j\in J\setminus\{i\}}d_{j}Y_{j}.
    \end{aeq}%
    Define $D=d_{i}Y_{i}$ and $X=\sum_{j\in J\setminus\{i\}}d_{j}Y_{j}$. Since $d_{i}$ is a nonzero field element and $Y_{i}$ is uniform and independent of $X$, $D$ and $X$ are mutually independent and uniform.  By \Cref{lem:indepsum}, $Y_0=D+X$ and $X$ are mutually independent, and thus $Y_0$ is independent of any subset that excludes share $i$, for any $i\in J$.

    Note that any subset with size less than $k-1$ is included in the sum $\sum_{j\in J\setminus\{i\}}d_{j}Y_{j}$.  The independence and uniformity of the term $d_{i}Y_{i}$ remains sufficient.
\end{proof}

\subsection{Polynomial hash function}

In this subsection, we use the following notations:
\begin{itemize}[leftmargin=0.5cm]
    \setlength\itemsep{0em}
    \item $y_{(j)}$ denotes the secret ($y_{0}$) from the $j$th of $3+m$ secret sharing schemes being run in parallel to build a $(3+m)$-element secret $Y^A_{0}$, which $j\in\{-2,-1,0,\dots,m\}$ indexes into. Set $c:=y_{(-2)}$, $d:=y_{(-1)}$ and $e:=y_{(0)}$.
    \item The differences $c'$, $d'$, $e'$ and $y'_{(j)}$ each correspond to $c$, $d$, $e$ and $y_{(j)}$ as the difference $y'_0$ for the $y_0$ in the proof of \cref{thm:shamir_linearity}.
\end{itemize}
Consider the family of functions defined by%
\begin{aeq}\label{eq:hash_family_2}
    \mbf{H}'=\{h'_{c,d,e}\colon& F^m\to F\colon\\
    &(y_{(1)},\dots,y_{(m)})\mapsto{}d+ce+\sum_{j=1}^{m}c^{j+1}y_{(j)}\},
\end{aeq}%
where $c$, $d$ and $e$ are elements of a finite field $F$.
Note that this is essentially the same family of functions as used for message hashing: the first element in the list has been shown as a subscript due to its role as a function-selection parameter, and a prime has been added to distinguish it. 

\begin{theorem}\label{thm:shamir_correctness}
    Denote $\mbf{y}=(y_{(1)},\dots,y_{(m)})$ and $\mbf{y}'=(y'_{(1)},\dots,y'_{(m)})$.
    Let $\Omega=F^3$ be a sample space with uniform probability.
    Let $h'_{C,D,E}(\mbf{y})=D+CE+\sum_{j=1}^{m}C^{j+1}y_{(j)}$ define a family of hash functions with random variables $(C,D,E)\in\Omega$ as selection parameters. Let $m\ne0.$
    Then, $\max_{t',c',d',e',\mbf{y}'\ne0} \Pr(t+t'=h'_{C+c',D+d',E+e'}(\mbf{y}+\mbf{y}')~|~t=h'_{C,D,E}(\mbf{y}))\le\min(\frac{m+1}{|F|},1)$.
\end{theorem}
\begin{proof}
    Given a Shamir secret sharing scheme used to transmit all of $C$, $D$, $E$ and $\mbf{y}$, an adversary who controls from $1$ to $k-1$ shares can modify $C$, $D$ and $E$ simultaneously by adding a chosen constant to each (as per \cref{thm:shamir_linearity}), with $t$ and $\mbf{y}$ assumed known and modifiable.  Thus, $t$, $C$, $D$, $E$ and $\mbf{y}$ are replaced with $t+t'$, $C+c'$, $D+d'$, $E+e'$ and $\mbf{y}+\mbf{y}'$ respectively.

    We are given that $t=h'_{C,D,E}(\mbf{y})$, which may be written%
    \begin{aeq}\label{eq:hash_shamir_given}
        t=D+CE+\sum_{j=1}^{m}C^{j+1}y_{(j)}.
    \end{aeq}%
    This determines a unique value $D$ for every pair of values $C,E$, and since the \textit{a priori} probability on $\Omega$ is uniform, the \textit{a posteriori} marginal distribution over pairs $(C,E)$ remains uniform, but the marginal distribution on $D$ is potentially nonuniform by a similar argument as in the proof of \cref{thm:message_correctness}.
    To obtain the probability that $t+t'=h'_{C+c',D+d',E+e'}(\mbf{y}+\mbf{y}')$ holds, we subtract the given \cref{eq:hash_shamir_given} from it to obtain the equivalent equation%
    \begin{aeq}\label{eq:hash_shamir_attack}
        t'=~&d'+c'E+Ce'+c'e'\\
        &+\sum_{j=1}^{m}[(C+c')^{j+1}(y_{(j)}+y'_{(j)})-C^{j+1}y_{(j)}].
    \end{aeq}%
    When $c'=0$ and $\mbf{y}'\ne0$, \cref{eq:hash_shamir_attack} reduces to%
    \begin{aeq}\label{eq:hash_shamir_reduced}
        t'=d'+Ce'+\sum_{j=1}^{m}C^{j+1}y'_{(j)},
    \end{aeq}%
    which is a non-constant polynomial in $C$ since $\mbf{y}'\ne0$ implies that for at least one value of $j$, $y'_{(j)}\ne0$, but is independent of $E$.  By the uniformity of $C$, each distinct root for the polynomial in $C$ has probability $\frac{1}{|F|}$. The number of distinct roots for a polynomial of degree $m+1$ is at most $\min(m+1,|F|)$, giving a maximum probability for \cref{eq:hash_shamir_reduced} holding of $\min(\frac{m+1}{|F|},1)$.

    When $c'\ne0$, \cref{eq:hash_shamir_attack} may reduce either to a non-constant or to a constant polynomial in $C$, but either way it retains the term that depends on $E$.  For the former (where there is a dependency on $C$), for each value of $E$ there may be up to $\min(m+1,|F|)$ values of $C$ that solve the polynomial, as for the case where $c'=0$, again giving a probability of holding of $\min(\frac{m+1}{|F|},1)$.  For the latter (where there is no dependency on $C$), \cref{eq:hash_shamir_attack} reduces to%
    \begin{aeq}\label{eq:hash_shamir_lincase}
        t'=~d'+c'E+c'e',
    \end{aeq}%
    which, by the uniformity of $E$ and that $c'\ne0$, has probability $\frac{1}{|F|}$ of holding.

    Given that $m$ cannot be negative, $\min(\frac{m+1}{|F|},1)\ge\frac{1}{|F|}$.  Thus, considering all the cases above, the maximum probability of \cref{eq:hash_shamir_attack} holding under the condition $\mbf{y}'\ne0$ is upper-bounded by $\min(\frac{m+1}{|F|},1)$.

    We exclude the case $m=0$, since the $\max$ operator over an empty domain is undefined.

    Thus, we have that for $m\ne0$,%
    \begin{aeq}
        \max_{t',c',d',e',\mbf{y}'\ne0} \Pr(t+t'=h'_{C+c',D+d',E+e'}(\mbf{y}+\mbf{y}')) \\
        \le\min\big(\frac{m+1}{|F|},1\big).
    \end{aeq}%
\end{proof}
