# Supplementary material for: Distributed Symmetric Key Establishment: a Scalable Quantum-Safe Key Distribution Protocol
Source: arXiv:2407.20969 source file (2024-07-30)
Supplement: Supplementary file 5 [file tests_and_results.tex]

\section{Experimental Tests \& Results} \label{app:results}

\subsection{DSKE Device Feasibility \& Performance Experiment}
\label{appsub:isc}

% \subsubsection{Details}
% \label{appsubsub:isc_details}

% The DSKE network was physically set up in two colocations, Montreal and Ottawa. The use of colocations was to simulate the need for these places to have a client entity generating keys in a secure way.

% The 3 Security Hubs, 2 located in AWS and one located in an Ottawa colocation, each consisted of 1 Local Distributor, from which PSRD would be sent (before PSRD delivery to a client), which were installed on standard laptops. ID Quantique's Quantis QRNG was plugged into the laptops to generate PSRD. Upon sending PSRD from Local Distributor to client, the Local Distributor would erase its copy, to minimize the number of PSRD duplicates floating around (increasing security).

\subsubsection{Results}
\label{appsubsub:isc_results}

Multiple different tests were ran, to test the performance, reliability, and security of the DSKE network. Results are summarized in \Cref{table:isc_results}.

\newcolumntype{S}{>{\centering\arraybackslash}m{4.5cm}}

\newcolumntype{D}{>{\centering\arraybackslash}m{3.2cm}}

\begin{table}[ht!]
    \caption{DSKE Device Experiment Tests and Results}
    \label{table:isc_results}
    \centering
    \begin{tabular}{|S|D|}
    \hline
    \makecell{
        \parbox{4.5cm}{
            \centering
            \textbf{Test \& Performance Indicator}
        }
    } & \makecell{
        \parbox{3.2cm}{
            \centering
            \textbf{Result}
        }
    } \\ 
    \hline
    \makecell{
        \parbox{4.5cm}{
            \begin{flushleft}
            \textbf{Information Theoretical Security} \\
            Enlist a security consulting party to verify the information-theoretical security of both DSKE encryption and authentication. \\
            \textbf{Performance Indicator}: A third party verifies DSKE design
            \end{flushleft}
        }
    } & \makecell{
        \parbox{3.2cm}{
            \begin{flushleft}
            The full DSKE proof was provided to a security consulting party, who confirmed that the protocol was of sound design and information-theoretically secure.
            \end{flushleft}
        }
    } \\
    \hline
    \makecell{
        \parbox{4.5cm}{
            \begin{flushleft}
            \textbf{Lack of Distance Limitations between Clients} \\
            By simply showing that the clients can communicate on mobile devices, requiring only an internet connection, it shows no distance limitations. \\
            \textbf{Performance Indicator}: Clients are able to communicate with an internet connection.
            \end{flushleft}
        }
    } & \makecell{
        \parbox{3.2cm}{
            \begin{flushleft}
            All clients were successfully onboarded and it was confirmed that they were able to communicate over the internet.
            \end{flushleft}
        }
    } \\
    \hline
    \makecell{
        \parbox{4.5cm}{
            \begin{flushleft}
            \textbf{Size Scalability} \\
            Onboard up to 5 mobile clients, one at a time, and show that
            \begin{enumerate}
                \item they can keep communicating.
                \item the onboarding process remains identical, and is independent of network size.
            \end{enumerate}
            \textbf{Performance Indicator}: Clients communicate continuously during onboarding, with no process changes.
            \end{flushleft}
        }
    } & \makecell{
        \parbox{3.2cm}{
            \begin{flushleft}
            While onboarding each of the mobile clients, 
            \begin{enumerate}
                \item existing clients were able to communicate.
                \item the onboarding process was identical for each client.
            \end{enumerate}
            \end{flushleft}
        }
    } \\
    \hline
    \makecell{
        \parbox{4.5cm}{
            \begin{flushleft}
            \textbf{Fault tolerance and no single point of failure} \\
            With 2 clients continually generating keys using 3 Security Hubs:
            \begin{enumerate}
                \item \textbf{Bring one Hub offline} 
                Key generation should continue.
                \item \textbf{Bring another Hub offline}  
                Key generation should cease.
            \end{enumerate}
            \textbf{Performance Indicator}: Key generation continues while $\ge$ 2 Hubs are online. 
            \end{flushleft}
        }
    } & \makecell{
        \parbox{3.2cm}{
            \begin{flushleft}
            With the 2 clients continually generating keys, 
            \begin{enumerate}
                \item when one hub was switched off, key generation continued.
                \item when another hub was switched off, key generation ceased.
            \end{enumerate}
            This behaviour was as expected.
            \end{flushleft}
        }
    } \\
    \hline
    \makecell{
         \parbox{4.5cm}{
            \begin{flushleft}
            \textbf{Black box penetration testing} \\
            A third party company was contracted to perform the pen test on the KME and DSKE client solution. \\
            \textbf{Performance Indicator}: KME and DSKE client solution passes test suite.
            \end{flushleft}
        }
    } & \makecell{
        \parbox{3.2cm}{
            \begin{flushleft}
            The third party company confirmed that the KME and DSKE client solution passed their black box penetration test suite.
            \end{flushleft}
        }
    } \\
    \hline
    \makecell{
        \parbox{4.5cm}{
            \begin{flushleft}
            \textbf{Performance} \\
            2 virtual DSKE clients operated in the cloud are created, and performance is measured by the maximum key rate attained in the test environment. \\
            \textbf{Performance Indicator}: Key generation rate exceeds 20 Mbit/s.
            \end{flushleft}
        }
    } & \makecell{
        \parbox{3.2cm}{
            \begin{flushleft}
            The 2 clients were able to exceed 20 Mbit/s of created DSKE key material between them.
            \end{flushleft}
        }
    } \\
    \hline
    \end{tabular}
\end{table}
